# Supplementary material for: Measuring Societal Biases from Text Corpora with Smoothed First-Order Co-occurrence
Source: arXiv:1812.10424 source file (2021-04-27)
Supplement: Supplementary file 1 [file main_appendix.tex]

%%
%% This is file `sample-sigconf.tex',
%% generated with the docstrip utility.
%%
%% The original source files were:
%%
%% samples.dtx  (with options: `sigconf')
%% 
%% IMPORTANT NOTICE:
%% 
%% For the copyright see the source file.
%% 
%% Any modified versions of this file must be renamed
%% with new filenames distinct from sample-sigconf.tex.
%% 
%% For distribution of the original source see the terms
%% for copying and modification in the file samples.dtx.
%% 
%% This generated file may be distributed as long as the
%% original source files, as listed above, are part of the
%% same distribution. (The sources need not necessarily be
%% in the same archive or directory.)
%%
%% The first command in your LaTeX source must be the \documentclass command.
\documentclass[sigconf]{acmart}

\usepackage{times,latexsym}
\usepackage[utf8]{inputenc} % allow utf-8 input
\usepackage[T1]{fontenc}    % use 8-bit T1 fonts
\usepackage{url}            % simple URL typesetting
\usepackage{booktabs}       % professional-quality tables
\usepackage{amsfonts}       % blackboard math symbols
\usepackage{nicefrac}       % compact symbols for 1/2, etc.
\usepackage{microtype}      % microtypography
\usepackage{booktabs} % For formal tables
\usepackage{times}
\usepackage{latexsym}
\usepackage{booktabs}
\usepackage{xspace}
\usepackage{amssymb}
\usepackage{dsfont}
\setcounter{tocdepth}{3}
\usepackage{multirow}
\usepackage{subfig}
\usepackage{amsmath}
\usepackage[prependcaption]{todonotes}
\usepackage{multirow}
\usepackage{graphicx,wrapfig,lipsum}
\usepackage{subfig}
\usepackage{csquotes}
\usepackage{xcolor}
\usepackage{fancyvrb}
\usepackage[export]{adjustbox}

\usepackage{arydshln}
\usepackage[markup=underlined]{changes}

\usepackage{xcolor,colortbl}
\usepackage{array}

\newcolumntype{L}[1]{>{\raggedright\let\newline\\\arraybackslash\hspace{0pt}}m{#1}}
\newcolumntype{C}[1]{>{\centering\let\newline\\\arraybackslash\hspace{0pt}}m{#1}}
\newcolumntype{R}[1]{>{\raggedleft\let\newline\\\arraybackslash\hspace{0pt}}m{#1}}

\makeatletter
\def\adl@drawiv#1#2#3{%
        \hskip.5\tabcolsep
        \xleaders#3{#2.5\@tempdimb #1{1}#2.5\@tempdimb}%
                #2\z@ plus1fil minus1fil\relax
        \hskip.5\tabcolsep}
\newcommand{\cdashlinelr}[1]{%
  \noalign{\vskip\aboverulesep
           \global\let\@dashdrawstore\adl@draw
           \global\let\adl@draw\adl@drawiv}
  \cdashline{#1}
  \noalign{\global\let\adl@draw\@dashdrawstore
           \vskip\belowrulesep}}
\makeatother

\usepackage{bm}
\input{dlbook_mathcommands}

%% Rights management information.  This information is sent to you
%% when you complete the rights form.  These commands have SAMPLE
%% values in them; it is your responsibility as an author to replace
%% the commands and values with those provided to you when you
%% complete the rights form.
\setcopyright{acmcopyright}
\copyrightyear{2021}
\acmYear{2021}
\acmDOI{}

%% These commands are for a PROCEEDINGS abstract or paper.
\acmConference[FAccT '21]{FAccT '21: ACM Conference on Fairness, Accountability, and Transparency}{}{}
\acmBooktitle{FAccT '21: ACM Conference on Fairness, Accountability, and Transparency}
\acmPrice{}
\acmISBN{}

%%
%% Submission ID.
%% Use this when submitting an article to a sponsored event. You'll
%% receive a unique submission ID from the organizers
%% of the event, and this ID should be used as the parameter to this command.
%%\acmSubmissionID{123-A56-BU3}

%%
%% The majority of ACM publications use numbered citations and
%% references.  The command \citestyle{authoryear} switches to the
%% "author year" style.
%%
%% If you are preparing content for an event
%% sponsored by ACM SIGGRAPH, you must use the "author year" style of
%% citations and references.
%% Uncommenting
%% the next command will enable that style.
%%\citestyle{acmauthoryear}

%\newcommand{\biasmeanSim}{\textsc{Mean}\xspace}
%\newcommand{\biasmeanCo}{\textsc{First-Avg}\xspace}

\definecolor{darkfemale}{HTML}{e66101}
\definecolor{darkmale}{HTML}{5e3c99}
\definecolor{lightfemale}{HTML}{fdb863}
\definecolor{lightmale}{HTML}{b2abd2}
\definecolor{gray}{HTML}{bdbdbd}
\definecolor{cadmiumgreen}{rgb}{0.0, 0.42, 0.24}

%%
%% end of the preamble, start of the body of the document source.
\begin{document}

\title{Gender Bias Measurement in Text Corpora with Smoothed First-Order Co-occurrence}

%%
%% The "author" command and its associated commands are used to define
%% the authors and their affiliations.
%% Of note is the shared affiliation of the first two authors, and the
%% "authornote" and "authornotemark" commands
%% used to denote shared contribution to the research.
%\author{Ben Trovato}
%\authornote{Both authors contributed equally to this research.}
%\email{trovato@corporation.com}
%\orcid{1234-5678-9012}
%\author{G.K.M. Tobin}
%\authornotemark[1]
%\email{webmaster@marysville-ohio.com}
%\affiliation{%
%  \institution{Institute for Clarity in Documentation}
%  \streetaddress{P.O. Box 1212}
%  \city{Dublin}
%  \state{Ohio}
%  \postcode{43017-6221}
%}

%\author{Navid Rekabsaz \\
%  Johannes Kepler University \\
%  \texttt{navid.rekabsaz@jku.at} \\\And
%  James Henderson \\
%  Idiap Research Institute \\
%  \texttt{james.henderson@idiap.ch} \\\AND
%  Robert West \\
%  EPFL \\
%  \texttt{robert.west@epfl.ch} \\\And
%  Allan Hanbury \\
%  TU Wien, Complexity Science Hub Vienna \\
%  \texttt{allan.hanbury@tuwien.ac.at} \\}

%%
%% By default, the full list of authors will be used in the page
%% headers. Often, this list is too long, and will overlap
%% other information printed in the page headers. This command allows
%% the author to define a more concise list
%% of authors' names for this purpose.
%\renewcommand{\shortauthors}{Trovato and Tobin, et al.}

%%
%% This command processes the author and affiliation and title
%% information and builds the first part of the formatted document.
\maketitle

\appendix
\input{X-appendix}

%\bibliography{references}
%\bibliographystyle{ACM-Reference-Format}

\end{document}
